# Supplementary material for: Open-Vocabulary Multi-Label Classification via Multi-Modal Knowledge Transfer
Source: arXiv:2207.01887 source file (2023-02-01)
Supplement: Supplementary file 1 [file prediction_supp.pdf]

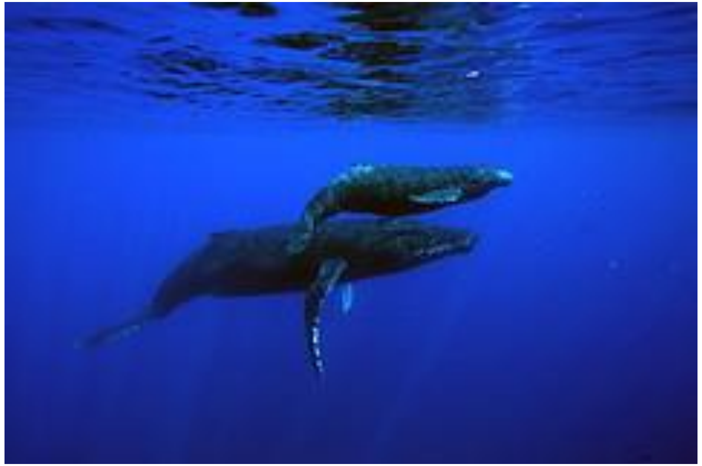

| First-Stage | Second-Stage |
|---|---|
| ocean | ocean |
| fish | fish |
| coral | whales |
| whales | water |
| animal | animal |

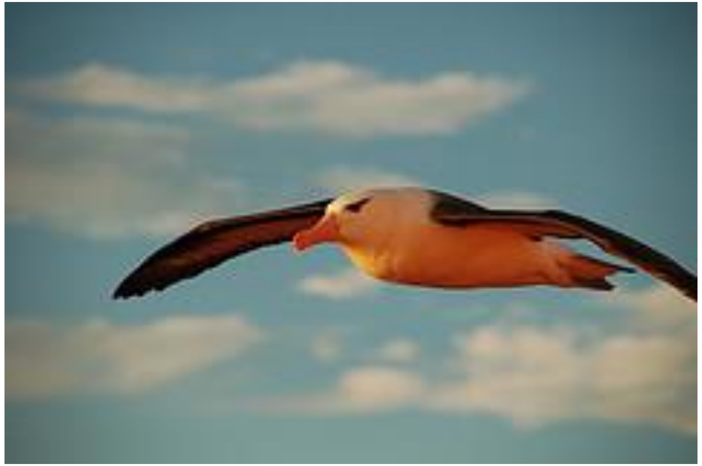

| First-Stage | Second-Stage |
|---|---|
| birds | birds |
| animal | animal |
| sky | sky |
| plane | plane |
| whales | clouds |

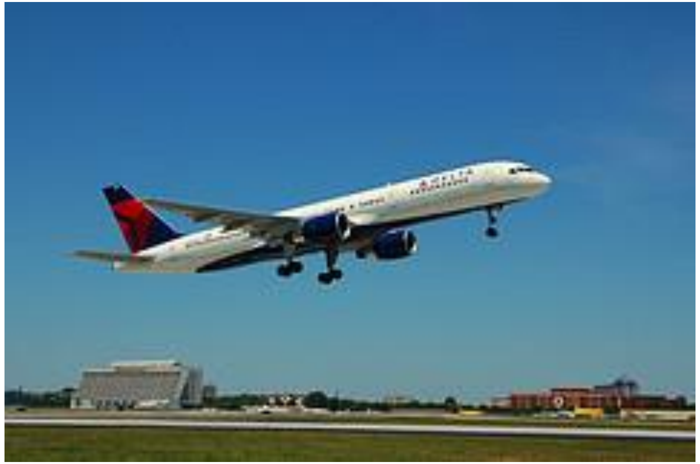

| First-Stage | Second-Stage |
|---|---|
| plane | plane |
| airport | airport |
| sky | sky |
| whales | birds |
| birds | clouds |

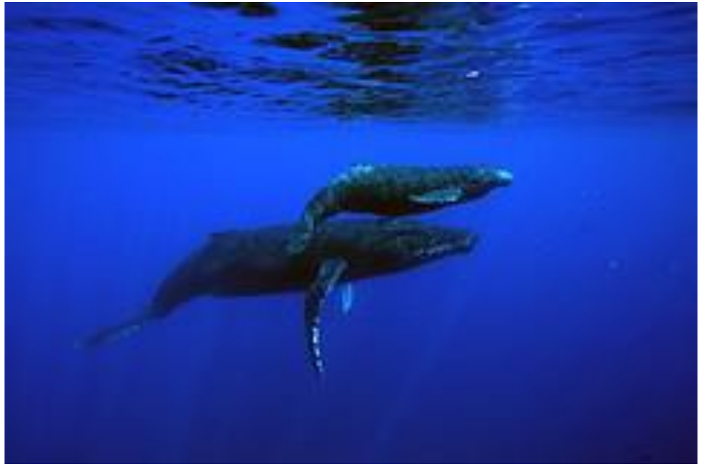

| w/o Prompt | w/ Prompt |
|---|---|
| ocean | ocean |
| fish | fish |
| coral | whales |
| whales | water |
| animal | animal |

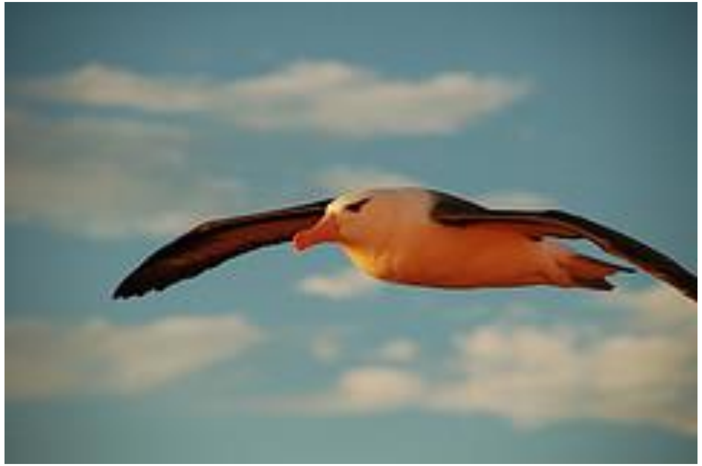

| w/o Prompt | w/ Prompt |
|---|---|
| birds | birds |
| animal | animal |
| sky | sky |
| plane | plane |
| whales | clouds |

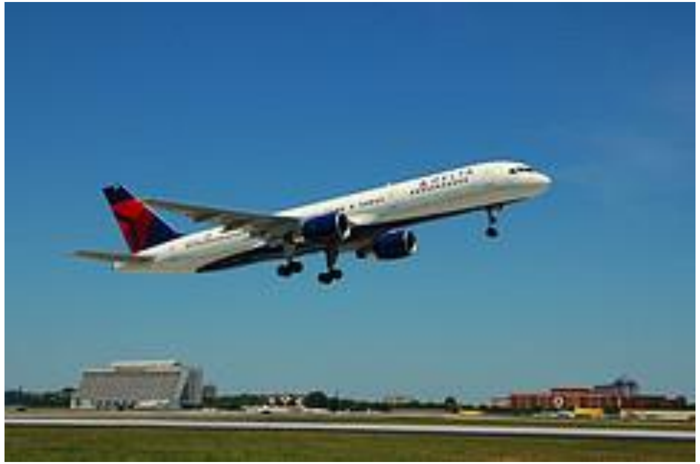

| w/o Prompt | w/ Prompt |
|---|---|
| plane | plane |
| airport | airport |
| sky | sky |
| whales | birds |
| birds | clouds |

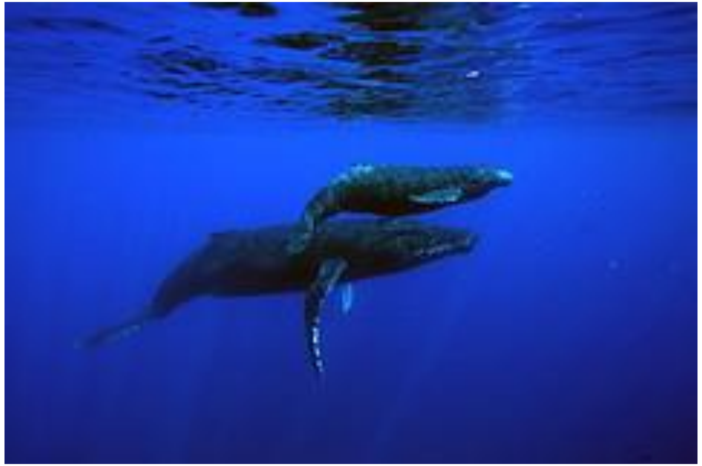

| w/o Tuning | w/ Tuning |
|---|---|
| ocean | ocean |
| fish | fish |
| coral | whales |
| whales | water |
| animal | animal |

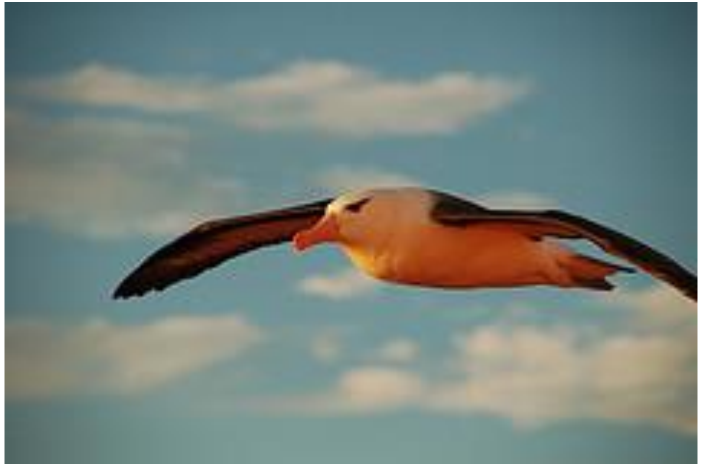

| w/o Tuning | w/ Tuning |
|---|---|
| birds | birds |
| animal | animal |
| sky | sky |
| plane | plane |
| whales | clouds |

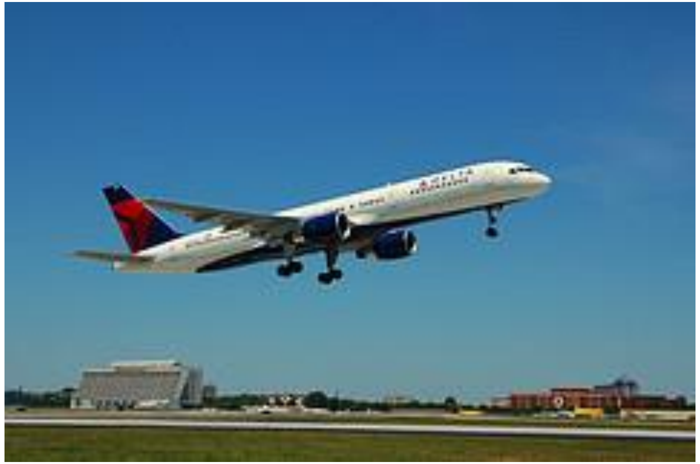

| w/o Tuning | w/ Tuning |
|---|---|
| plane | plane |
| airport | airport |
| sky | sky |
| whales | birds |
| birds | clouds |
